# Supplementary material for: A stable added-mass partitioned (AMP) algorithm for elastic solids and incompressible flow
Source: arXiv:1812.05208 source file (2018-12-13)
Supplement: Supplementary file 1 [file analysisAppendix.tex]

\section{Stability analysis details} \label{sec:StabilityAnalysisDetails}

\subsection{CFL region for Cauchy scheme} \label{sec:CFLRegionCauchy}

\das{Equation \eqref{eq:evProblem}.
For a range of values in the
$\lx-\ly$ plane, the maximum amplification factor over $\omega \in [0,2\pi]$ 
was computed numerically to determine the region where $|A| \le 1.$ }

{
\newcommand{\figWidth}{8cm}
\begin{figure}[h]
\begin{center}
\includegraphics[width=\figWidth]{fig/MaximumAmpForCauchyProblemSurf.png}
\includegraphics[width=\figWidth]{fig/MaximumAmpForCauchyProblemCont.png}
\caption{Left: surface plot of the maximum amplification factor, $|A|$
over $\omega \in [0,2 \pi]$ for the Cauchy problem. 
Right: the green fill indicates the stability region $|A| \le 1.$ 
The dotted line represents the curve $\lx^2 + \ly^2 = 1,$ which is contained in 
the region.}
\end{center}
\end{figure}
}
\subsection{Components of $\dMat$} \label{sec:ComponentsOfDmat}

Equation \eqref{eq:StabilitySystem} represents the system of equations that
arise when analyzing the stability of the simplified model problem.
The components of $\dMat$ can be obtained by substituting the normal mode ansatz into
the solid boundary conditions (ie. equation \eqref{eq:interfaceBCsForSolid}).
The first row of $\dMat$ is associated with boundary condition on the 
incoming characteristic.
For the AMP algorithm, this components of this row are defined as
\begin{align}
g_{1\nn, \;\text{AMP}} &= \frac{\beta_{2,\nn} M^2 + \beta_{1,\nn} M + \beta_{0,\nn} }
{\left(A^2 - \frac{4}{3} A + \frac{1}{3}\right) M^2
+ A^2 M + A^2} ,
\end{align}
where
\begin{align}
\beta_{0,\nn} &= A^2 \left(\qn{\nn} - \rn{\nn} - \qn{\nn} \left( \p_\nn + \frac{1}{\p_\nn} \right) \right),\\
\beta_{1,\nn} &= -A^2 \left( \frac{\qn{\nn}}{6} - \frac{5 \rn{\nn}}{6} 
+ \qn{\nn} \left(\p_\nn + \frac{1}{\p_\nn} \right)\right)
+ 2 A (\qn{\nn} - \rn{\nn})
+ \frac{1}{2} (\rn{\nn} - \qn{\nn}), \\
\beta_{2,\nn} &= \left(A^2 - \frac{4}{3} A + \frac{1}{3}\right)
\left(\qn{\nn} + \rn{\nn} - \qn{\nn} \left( \p_\nn + \frac{1}{\p_\nn}\right) \right) .
\end{align}
Similar expressions can be obtained for the TP and ATP algorithms. These expressions are 
given by
\begin{align}
\dComp_{1\nn, \;\text{TP}} &= 
(\rn{\nn} +\qn{\nn}) \left(\p_\nn + \frac{1}{\p_\nn} \right)
- M \frac{3A^2-4A+1}{A^2} (\rn{\nn}-\qn{\nn}),
\quad \nn=1,2, \\
\dComp_{1\nn, \;\text{ATP}} &= 
(\rn{\nn} -\qn{\nn}) \left(\p_\nn + \frac{1}{\p_\nn} \right)
- \frac{1}{4 M} \frac{A^2}{3A^2 - 4A + 1} (\rn{\nn} + \qn{\nn}),
\quad \nn=1,2.
\end{align}
The second row of 
$\dMat$ is common to all algorithms and represents 
extrapolation of the $\cp^+$ characteristic into the interface
ghost point. The second row is defined as
\begin{align}
\dComp_{2\nn} = \rn{\nn} \left(\p_\nn - 2 + \frac{1}{\p_\nn} \right), \quad \nn = 1,2.
\end{align}
